# Supplementary material for: Not-So-Optimal Transport Flows for 3D Point Cloud Generation
Source: arXiv:2502.12456 source file (2025-02-18)
Supplement: Supplementary file 1 [file procedure_details.tex]

\section{OT Approximation procedure.}

- What is OT distance
- Entropy regulaized formulation
- Sinkhorn divergence
- Algorithm
